# Supplementary material for: Quantification of finite-temperature effects on adsorption geometries of $\pi$-conjugated molecules
Source: arXiv:1405.3670 source file (2014-05-14)
Supplement: Supplementary file 1 [file AB-supplement_arXiv.pdf]

published in Phys. Rev. B **88**, 035421 (2013) DOI: 10.1103/PhysRevB.88.035421

# Supplementary Material to:

# Quantification of finite-temperature effects on adsorption geometries of $\pi$-conjugated molecules

G. Mercurio,[1,2,*] R. J. Maurer,[3] W. Liu,[4] S. Hagen,[5] F. Leyssner,[5] P. Tegeder,[5,6] J. Meyer,[3] A. Tkatchenko,[4] S. Soubatch,[1,2] K. Reuter,[3] and F. S. Tautz[1,2]

[1]*Peter Grünberg Institut (PGI-3), Forschungszentrum Jülich, 52425 Jülich, Germany*

[2]*Jülich Aachen Research Alliance (JARA), Fundamentals of Future Information Technology, 52425 Jülich, Germany*

[3]*Department Chemie, Technische Universität München, Lichtenbergstr. 4, 85747 Garching, Germany*

[4]*Fritz-Haber-Institut der Max-Planck-Gesellschaft, Faradayweg 4-6, 14195 Berlin, Germany*

[5]*Freie Universität Berlin, Fachbereich Physik, Arnimallee 14, 14195 Berlin, Germany*

[6]*Physikalisch-Chemisches Institut, Ruprecht-Karls-Universität Heidelberg, Im Neuenheimer Feld 253, 69120 Heidelberg, Germany*

(Dated: May 14, 2014)

## DFT CALCULATIONS

### Computational Details

All GGA-DFT supercell calculations [2, 3] were performed with the pseudopotential plane wave code CASTEP-6.0 [4, 5] using standard library ultrasoft pseudopotentials [6]. Short-range electronic exchange and correlation were treated on the gradient-corrected level using the PBE functional [7]. The lack of van der Waals interactions in semi-local exchange correlation functionals was corrected by semi-empirical pairwise dispersion correction schemes [8–10], namely the TS scheme [8] and the vdW$^{\mathrm{surf}}$ scheme [10]. The second one was specifically designed for use in adsorbate-substrate interactions. It accounts for the non-local collective substrate response via renormalization of the underlying parameters. All calculations were

TABLE I. List of cells used to calculate different coverages of adsorbed AB overlayers on the Ag(111) surface at $T = 0$ K. $n$: number of AB molecules per cell; $k$-grid: Monkhorst-Pack [1]; area/AB: surface area per AB molecule; $E_{\mathrm{ads}}$ (TS): adsorption energy *per molecule* and adsorption energy *per surface area* calculated with PBE+TS; $E_{\mathrm{ads}}$ (vdW$^{\mathrm{surf}}$): adsorption energy *per molecule* and adsorption energy per surface area calculated with PBE+vdW$^{\mathrm{surf}}$.

| cell | n | k-grid | area/AB (Å$^2$) | $E_{\mathrm{ads}}$ (TS) (eV) | (eV/nm$^2$) | $E_{\mathrm{ads}}$ (vdw$^{\mathrm{surf}}$) (eV) | (eV/nm$^2$) |
|---|---|---|---|---|---|---|---|
| 6×7 | 1 | 4×4×1 | 359.6 | 1.67 | 0.47 | 1.72 | 0.48 |
| 5×6 | 1 | 4×6×1 | 256.8 | 1.68 | 0.65 | 1.71 | 0.67 |
| 3×6 | 1 | 6×4×1 | 154.1 | 1.70 | 1.10 | 1.76 | 1.14 |
| 3×5 | 1 | 8×4×1 | 128.4 | 1.74 | 1.35 | 1.76 | 1.37 |
| 2×5 | 1 | 8×4×1 | 85.6 | 1.46 | 1.71 | 1.33 | 1.55 |
| 5×5 | 3 | 4×4×1 | 71.3 | 1.26 | 1.76 | 1.07 | 1.50 |
| 3×5 | 2 | 8×4×1 | 64.2 | 1.16 | 1.80 | 0.94 | 1.47 |
| 4×5 | 3 | 6×4×1 | 57.1 | 1.38 | 2.43 | 1.20 | 2.10 |
| 5×5 | 4 | 4×4×1 | 53.5 | 1.39 | 2.60 | 1.21 | 2.25 |
| 2×5 | 2 | 8×4×1 | 42.8 | 0.69 | 1.60 | 0.54 | 1.27 |

TABLE II. Geometry parameters of AB calculated with PBE+TS and PBE+vdW$^{surf}$ for each cell at $T = 0$ K. $d_{N-Ag}$: average adsorption height of N atoms above the surface Bragg plane; $d_{N_1-N_2}$: difference of the adsorption heights of the two N atoms within the AB molecule, i.e. $d_{N_1-N_2} = d_{N_1-Ag} - d_{N_2-Ag}$; $\omega$, $\beta$, $\beta'$, $\beta''$: dihedral angles, see supplement text and paper for definitions; $\langle d_{Ag} \rangle$: average distance of the Ag surface atoms from the surface Bragg plane. In case of cells with more than one AB molecule per cell, the listed geometry parameters refer to the average over all molecules in the cell.

| | | | TS | | | | | vdw$^{surf}$ | | | | | TS/vdw$^{surf}$ |
|---|---|---|---|---|---|---|---|---|---|---|---|---|---|
| cell | area/AB (Å$^2$) | AB/area (nm$^{-2}$) | $d_{N-Ag}$ (Å) | $d_{N_1-N_2}$ (Å) | $\omega$ (deg) | $\beta$ (deg) | $\beta'/\beta''$ (deg) | $d_{N-Ag}$ (Å) | $d_{N_1-N_2}$ (Å) | $\omega$ (deg) | $\beta$ (deg) | $\beta'/\beta''$ (deg) | $\langle d_{Ag} \rangle$ (Å) |
| $(6\times7)_1$ | 359.6 | 0.28 | 2.95 | 0.00 | 1.8 | -0.6 | -0.4/-0.9 | 2.61 | 0.02 | 4.5 | -2.0 | -1.7/-2.3 | 0.0000 |
| $(5\times6)_1$ | 256.8 | 0.39 | 2.96 | 0.00 | 2.8 | -1.2 | -1.2/-1.1 | 2.63 | 0.02 | 4.3 | -2.1 | -2.0/-2.2 | 0.0000 |
| $(3\times6)_1$ | 154.1 | 0.65 | 2.97 | 0.00 | 1.0 | -0.7 | -0.2/-1.2 | 2.58 | 0.01 | 5.0 | -1.8 | -1.5/-2.2 | -0.0181 |
| $(3\times5)_1$ | 128.4 | 0.78 | 2.95 | 0.01 | 3.0 | -1.2 | -1.3/-1.1 | 2.61 | 0.02 | 4.7 | -2.4 | -2.2/-2.5 | -0.0184 |
| $(2\times5)_1$ | 85.6 | 1.17 | 3.26 | 0.00 | 7.5 | 18.6 | 16.6/20.6 | 2.81 | 0.00 | 11.7 | 15.4 | 13.0/17.8 | -0.0186 |
| $(5\times5)_3$ | 71.3 | 1.40 | 3.56 | 0.14 | 12.8 | 32.4 | 28.8/36.0 | 3.47 | 0.04 | 11.3 | 34.2 | 31.1/37.3 | -0.0185 |
| $(3\times5)_2$ | 64.2 | 1.56 | 3.52 | 0.21 | 15.8 | 39.8 | 35.2/44.3 | 3.56 | 0.23 | 13.7 | 41.7 | 37.7/45.8 | -0.0184 |
| $(4\times5)_3$ | 57.1 | 1.75 | 4.40 | 1.06 | -6.8 | -26.2 | -24.6/-27.8 | 4.32 | 1.14 | -6.8 | -25.8 | -24.2/-27.4 | -0.0186 |
| $(5\times5)_4$ | 53.5 | 1.87 | 4.48 | 1.11 | -5.1 | -20.4 | -19.0/-21.7 | 4.39 | 1.07 | -5.1 | -20.2 | -18.9/-21.6 | -0.0185 |
| $(2\times5)_2$ | 42.8 | 2.34 | 5.47 | 1.42 | -0.7 | -0.4 | -0.3/-0.6 | 5.39 | 1.42 | -0.7 | -0.9 | -0.8/-1.0 | -0.0186 |

TABLE III. Geometry parameters of AB in a $(2x5)_1$ cell (phase A) after correcting for anharmonic effects at 210 K ($\mathbf{R}_{210K}$), calculated with PBE+TS and PBE+vdw$^{surf}$.

| | $d_{N-Ag}$ (Å) | $d_{N_1-N_2}$ (Å) | $\omega$ (deg) | $\beta$ (deg) | $\beta'/\beta''$ (deg) | $\langle d_{Ag}\rangle$ (Å) |
|---|---|---|---|---|---|---|
| TS | 3.23 | 0.05 | 8.8 | 17.3 | 15.6/18.9 | -0.0186 |
| vdw$^{surf}$ | 2.98 | 0.01 | 9.0 | 17.7 | 16.0/19.4 | -0.0186 |

performed with frozen (111) 4 layer surface slabs of fcc Ag (with lattice constant $a = 4.14$ Å) with a 350 eV plane wave cutoff. Spin polarization was not taken into account. The vacuum was chosen to exceed 20 Å.

We used a variety of different surface slabs with a varying number of molecules, in order to simulate different AB coverages. Table I shows the cells taken into consideration, as well as the different number of $k$-points used [1]. The $k$-point and energy cutoff settings were chosen to guarantee convergence with respect to those parameters.

The electronic structure was converged to a total energy difference of $10^{-8}$eV. Convergence was eased with a Gaussian smearing of 0.15 eV. Molecular geometries were generated by sequential constrained geometry optimization [11] down to a maximum force component of 25 meV/Å per atom, an energy difference criterion of $2 \times 10^{-5}$eV per atom and a maximum step size of $10^{-3}$Å.

The adsorption energies of AB in each cell and the corresponding adsorption energies per surface area calculated with PBE+TS and PBE+vdW$^{surf}$ are reported in Table I. The corresponding geometry parameters are reported in Table II. For a definition of the dihedral angles $\omega$ and $\beta$, see paper. Since the DFT-calculated geometries have nonplanar phenyl rings (for $\omega \neq 0°$), two additional dihedral angles are defined, $\beta'$ ($C_1C_0NN$) and $\beta''$ ($C_2C_0NN$), where $C_0$ is the C atom bound to N, $C_1$ and $C_2$ are the two C atoms bound to $C_0$.

### Anharmonic correction to the AB geometry

To determine the average AB geometry at 210 K in the $(2{\times}5)_1$ cell ($\mathbf{R}_{210K}$) the following steps were followed. Note that all DFT calculations in the procedure described below were

performed using separately PBE+TS and PBE+vdW$^{\mathrm{surf}}$.

***Step 1:*** Normal modes were calculated for the DFT-calculated 0 K geometry of AB/Ag(111) in the $(2{\times}5)_1$ cell that is given by the 24×3-dimensional position vector $\mathbf{R}_0$. The following steps 2 to 5 were carried out for each harmonic mode with frequency $\nu_i$ $(i = 1, \ldots, 72)$ and displacement eigenvector $\mathbf{e}_i = \left(\frac{1}{\sqrt{m_1}}\tilde{\mathbf{e}}_i^1, \ldots, \frac{1}{\sqrt{m_{24}}}\tilde{\mathbf{e}}_i^{24}\right)$. $\tilde{\mathbf{e}}_i^I$ $(I = 1, \ldots, 24)$ are three-dimensional displacement vectors of the individual AB atoms, mass-weighted by $\sqrt{m_I}$ with the corresponding atomic masses $m_I$, such that the 72 vectors $(\tilde{\mathbf{e}}_i^1, \ldots, \tilde{\mathbf{e}}_i^{24})$ form an orthonormal set.

***Step 2:*** $\mathbf{R}_0$ was displaced along $\mathbf{e}_i$ and $-\mathbf{e}_i$ by the average mode amplitude $\langle \mathrm{A}_i \rangle$ at $T = 210$ K:

$$\langle \mathrm{A}_i \rangle = \frac{\sqrt{2k_{\mathrm{B}}T}}{\nu_i}, \tag{1}$$

with $k_{\mathrm{B}}$ equal to the Boltzmann constant, providing the two respective geometries $\mathbf{R}_0 + \langle \mathrm{A}_i \rangle \mathbf{e}_i$ and $\mathbf{R}_0 - \langle \mathrm{A}_i \rangle \mathbf{e}_i$. Analogously, two additional AB geometries, $\mathbf{R}_0 + \frac{\langle \mathrm{A}_i \rangle}{2}\mathbf{e}_i$ and $\mathbf{R}_0 - \frac{\langle \mathrm{A}_i \rangle}{2}\mathbf{e}_i$, were constructed.

***Step 3:*** For each of the above AB geometries $\mathbf{R}_0 + \Delta\mathbf{R}_i$ (with $\Delta\mathbf{R}_i = -\langle \mathrm{A}_i \rangle \mathbf{e}_i$, $-\frac{\langle \mathrm{A}_i \rangle}{2}\mathbf{e}_i$, 0, $+\frac{\langle \mathrm{A}_i \rangle}{2}\mathbf{e}_i$, $+\langle \mathrm{A}_i \rangle \mathbf{e}_i$) the corresponding DFT energy $E^{\mathrm{DFT}}(\mathbf{R}_0 + \Delta\mathbf{R}_i)$ was calculated.

***Step 4:*** The resulting five data points $E^{\mathrm{DFT}}(\mathbf{R}_0 + \Delta\mathbf{R}_i)$ were fitted with a Morse potential [12]:

$$V_i(r_i) = D_i \left[1 - \exp(-a_i r_i)\right]^2, \tag{2}$$

where $r_i$ is the (mass-weighted) displacement from the equilibrium, $D_i$ and $a_i$ describe respectively the depth of the potential and its curvature at the minimum. Going one step beyond the harmonic regime, the vibrational modes are thus represented by an uncoupled set of anharmonic potentials $V_i(r_i)$.

***Step 5:*** The equation of motion in each Morse potential $V_i(r_i)$ was integrated over one period $\mathrm{T}_i$. For energies $E$ smaller than $D_i$, the equation of motion of the Morse potential

$V_i\left(r_i\right)$ is [12]:

$$a_i r_i\left(t\right) = \log\left[\frac{1-\cos\theta\cos\left(2\pi\nu_i t\sin\theta\right)}{\sin^2\theta}\right], \tag{3}$$

where $\theta$ is the phase angle determined by the initial conditions (with $\cos^2\theta = E/D_i$), $t$ is the time variable and $E = k_\mathrm{B}T = 18$ meV at $T = 210$ K. As a result of the integration we obtained $\langle r_i\rangle$ which deviates more from 0 the stronger is the anharmonicity. $\mathbf{R}_0 + \langle r_i\rangle\mathbf{e}_i$ is the time-averaged AB geometry at 210 K if only mode $i$ was active.

***Step 6:*** The average AB geometry at 210 K ($\mathbf{R}_{210\mathrm{K}}$) with all the possible modes active was calculated by adding all time-averaged displacements to the 0 K geometry:

$$\mathbf{R}_{210\mathrm{K}} = \mathbf{R}_0 + \sum_{i=1}^{72}\langle r_i\rangle\mathbf{e}_i. \tag{4}$$

We found *a posteriori* that only modes with energies below 100 meV contribute significantly to the sum in equation (4). $\mathbf{R}_{210\mathrm{K}}$ is the finite-temperature DFT geometry which is compared in the paper to the NIXSW-determined experimental geometry. The NIXSW simulations of the average geometry $\mathbf{R}_{210\mathrm{K}}$ are reported in Section . The corresponding geometry parameters are reported in Table III.

## NIXSW: RESULTS AND SIMULATIONS

### NIXSW data analysis

For the general procedure followed here to analyze NIXSW data in order to determine the structure parameters ($P_c$, $F_c$) and the corresponding error bars we refer to Ref. [13]. In brief, an NIXSW data set consists of all the core-level x-ray photoemission (PE) spectra recorded during one NIXSW experiment as the photon energy of the incoming x-ray beam is scanned through the Bragg condition ($E_\mathrm{Bragg} = 2634$ eV). Each PE spectrum is fitted by the software CasaXPS [14] in order to determine the corresponding PE yield, i.e. the area of the whole PE spectrum (or of one or more components thereof) after background subtraction. The fitting models of Ag3$d$, C1$s$ and N1$s$ PE spectra are reported in Ref. [15, 16]. The corresponding PE yield profiles (PE yield vs. photon energy) are fitted by the program Torricelli [15, 17, 18], and results are reported in Ref. [15, 16]. A detailed description

of NIXSW data analysis of AB/Ag(111), including an extensive presentation of NIXSW simulations (summarized in Sections  and ), is the subject of a forthcoming publication [16]. Therein, NIXSW results, including refined geometry determination, of another large organic molecular switch, 3,3′,5,5′-tetra-*tert*-butyl-azobenzene (TBA), adsorbed on Ag(111), will be reported.

Since experiments were carried out at 210 K we had to account for thermal contraction of the Ag crystal. The Ag lattice constant at 293 K is $a_{293\,\mathrm{K}} = 4.08641$ Å, Ref. [19]). From the Ag thermal expansion coefficient at 200 K, $\epsilon_{200\,\mathrm{K}} = -1.720 \times 10^{-3}$ (Ref. [20]), we obtain $a_{210\,\mathrm{K}} \approx a_{200\,\mathrm{K}} = a_{293\,\mathrm{K}} + a_{293\,\mathrm{K}}\epsilon_{200\,\mathrm{K}} = 4.07938$ Å. Hence, at 210 K we obtain a Bragg spacing $d_{\mathrm{Ag}(111)} = a_{210\,\mathrm{K}}/\sqrt{3} = 2.3552$ Å. The corresponding Bragg energy is $E_{\mathrm{Bragg}} = 2634$ eV.

We note that, although in this paper the focus is more on the hitherto generally neglected vibrations of the adsorbate, we also took the vibrations of the Ag substrate atoms into account. This was implemented by including the corresponding Debye-Waller factor $\exp(-M) = 0.9727$ (Ref. [15]), where $M$ is a temperature-dependent parameter calculated according to the formulas in Ref. [21] with $T = 210$ K. The Debye-Waller factor multiplies the Ag atomic scattering factor and it is thus implicitly contained in the reflectivity curve that enters directly the fitting function of the PE yield profiles [15, 18]. The physical effect of vibrations of the substrate atoms is to reduce the diffracted beam intensity, to decrease the coherence of the standing wave field, and thus to decrease $F_c$ of all species by the Debye-Waller factor, without however affecting the coherent positions $P_c$s (Ref. [22]). The influence of the adsorbate vibrations on the structure parameters ($P_c$, $F_c$) therefore comes on top of the influence of the substrate vibrations, and both are taken into account here.

**Comparison with previous NIXSW results**

Compared to the structure parameters ($P_c$, $F_c$) published in Ref. [23], slightly different structure parameters are quoted in this work (cf. the text of the paper). This refinement of the structure parameters was achieved in the following way:

(1) In Ref. [23] the binding energy window in which the photoemission spectra are fitted is adjusted for each spectrum in order to improve the fit. In the present work, the binding energy window is kept constant, because this procedure is more reproducible.

(2) In the present work, we use nondipolar correction parameters calculated according

TABLE IV. Nondipolar parameters $Q$, $\Delta$ and $S_R$, $|S_I|$, $\Psi$ calculated for C1$s$ and N1$s$ lines according to formulas in Refs. [24, 25] $\gamma$ is the angular distribution parameter [26]. $\delta_p$ and $\delta_d$ are the scattering phase shifts for p- and d- asymptotic waves, available from ab initio calculations [27].

| | $\gamma$ | $\delta_p$ | $\delta_d$ | $Q$ | $\Delta$ | $S_R$ | $\|S_I\|$ | $\Psi$ |
|---|---|---|---|---|---|---|---|---|
| C1$s$ | 1.061 | 0.7993 | 0.5879 | 0.250 | −0.211 | 1.667 | 1.336 | −0.054 |
| N1$s$ | 1.022 | 0.9074 | 0.6553 | 0.241 | −0.252 | 1.635 | 1.320 | −0.062 |

to formulas in Refs. [24, 25] (Table IV), instead of values based on measurements (as in Ref. [23]) that may lead to ambiguous results [28–30].

(3) In the present work, NIXSW data were analyzed with the program TORRICELLI [15, 17, 18] which is based on a different fitting function for the PE yield and a different fitting algorithm compared to the program DARE that was employed in Ref. [23].

### Calculation of structure parameters ($P_c$, $F_c$) for a given distribution of atoms

Consider an atomic species X. Assume that $N_{\mathrm{X}}$ atoms $\mathrm{X}_i$ ($i = 1, \ldots, N_{\mathrm{X}}$) are distributed across a Bragg spacing. This distribution is defined by the individual coherent positions $P_c^{\mathrm{X}_i}$ of these atoms. The $P_c^{\mathrm{X}_i}$ can be calculated from the corresponding vertical positions with respect to the nearest underlying Bragg plane $d_{\mathrm{X}_i}$ as[13]:

$$P_c^{\mathrm{X}_i} = \frac{d_{\mathrm{X}_i} \bmod d_{\mathbf{H}}}{d_{\mathbf{H}}}, \tag{5}$$

where $d_{\mathbf{H}}$ is the Bragg spacing of the $\mathbf{H} = (h, k, l)$ reflection. The corresponding coherent fraction of atom $\mathrm{X}_i$ is

$$F_c^{\mathrm{X}_i} = \frac{1}{N_{\mathrm{X}}}. \tag{6}$$

Using the Fourier notation, $P_c^{\mathrm{X}_i}$ and $F_c^{\mathrm{X}_i}$ can be interpreted as the phase and the amplitude of the Fourier vector

$$\tilde{f}_{\mathbf{H}}^{\mathrm{X}_i} = F_c^{\mathrm{X}_i} \exp\left(2\pi i P_c^{\mathrm{X}_i}\right). \tag{7}$$

Therefore, the Fourier vector representing the complete distribution of atoms of species X is given by the sum of all individual vectors

$$\tilde{f}_{\mathbf{H}}^{\mathrm{X}} = \sum_{i=1}^{N_{\mathrm{X}}} \tilde{f}_{\mathbf{H}}^{\mathrm{X}_i} = \Re \tilde{f}_{\mathbf{H}}^{\mathrm{X}} + \Im \tilde{f}_{\mathbf{H}}^{\mathrm{X}} = F_c^{\mathrm{X}} \exp\left(2\pi i P_c^{\mathrm{X}}\right), \tag{8}$$

where

$$\Re \tilde{f}_{\mathbf{H}}^{\mathrm{X}} = \sum_{i=1}^{N_{\mathrm{X}}} \Re \tilde{f}_{\mathbf{H}}^{\mathrm{X}_i} = \sum_{i=1}^{N_{\mathrm{X}}} F_c^{\mathrm{X_i}} \cos\left(2\pi P_c^{\mathrm{X_i}}\right), \tag{9}$$

$$\Im \tilde{f}_{\mathbf{H}}^{\mathrm{X}} = \sum_{i=1}^{N_{\mathrm{X}}} \Im \tilde{f}_{\mathbf{H}}^{\mathrm{X}_i} = \sum_{i=1}^{N_{\mathrm{X}}} F_c^{\mathrm{X_i}} \sin\left(2\pi P_c^{\mathrm{X_i}}\right). \tag{10}$$

Hence, the coherent position and fraction of the distribution of species X are given by

$$P_c^{\mathrm{X}} = \frac{1}{2\pi} \times \begin{cases} \arctan\left(\Im \tilde{f}_{\mathbf{H}}^{\mathrm{X}} / \Re \tilde{f}_{\mathbf{H}}^{\mathrm{X}}\right) & \Re \tilde{f}_{\mathbf{H}}^{\mathrm{X}} > 0 \\ \arctan\left(\Im \tilde{f}_{\mathbf{H}}^{\mathrm{X}} / \Re \tilde{f}_{\mathbf{H}}^{\mathrm{X}}\right) + \pi & \Re \tilde{f}_{\mathbf{H}}^{\mathrm{X}} < 0 \end{cases}, \tag{11}$$

and

$$F_c^{\mathrm{X}} = \sqrt{\left[\Re \tilde{f}_{\mathbf{H}}^{\mathrm{X}}\right]^2 + \left[\Im \tilde{f}_{\mathbf{H}}^{\mathrm{X}}\right]^2}. \tag{12}$$

**Calculation of geometry parameters ($\omega, \beta$) from measured structure parameters ($P_c$, $F_c$)**

In this section we address the following question: Which geometry parameters $(\omega, \beta)$ of AB are consistent with a given set of measured structure parameters ($P_c$, $F_c$)? In other words, we want to deduce the internal geometry of the AB molecule from the measured NIXSW data. The determination of $\omega$ and $\beta$ proceeds in the following steps:

***Step 1:*** For all possible combinations of dihedral angles ($\omega$,$\beta$) the coordinates of all atoms of AB are calculated.

***Step 2:*** The nitrogen atoms of AB are fixed at the experimental adsorption height $d_{\mathrm{N-Ag}}$, which follows directly from the measured structure parameters ($P_c^{\mathrm{N}}$, $F_c^{\mathrm{N}}$)|(exp). Then for each AB geometry the ($P_c^{\mathrm{C}}$, $F_c^{\mathrm{C}}$)|($\omega$,$\beta$) are calculated from the atomic coordinates of step 1 following the procedure defined in section  of the present supplement.

***Step 3:*** The crossing of ($P_c^{\mathrm{C}}$, $F_c^{\mathrm{C}}$)|($\omega$,$\beta$) with the measured ($P_c^{\mathrm{C}}$, $F_c^{\mathrm{C}}$)|(exp) provides the experimental geometry parameters ($\omega$,$\beta$)|(exp) (cf. Fig. 2 of the paper).

In the following, detailed information for each step is given.

***Ad step 1:*** AB geometries with any combination of $\omega$ and $\beta$ (with $0° \leq \omega \leq 360°$, $\Delta\omega = 1°$, $0° \leq \beta \leq 360°$, $\Delta\beta = 1°$) were generated using the program package Torricelli [15, 17, 18].

***Ad step 2:*** $d_{\mathrm{N-Ag}}$ is calculated using equation 5. Given the experimental value $P_c^{\mathrm{N}} = 0.26$ and $d_{\mathbf{H}} = 2.3552$ Å, the most plausible $d_{\mathrm{N-Ag}}$ is $\left(1 + P_c^{\mathrm{N}}\right) d_{\mathbf{H}} = 2.97$ Å. In fact, both $P_c^{\mathrm{N}} d_{\mathbf{H}} = 0.61$ Å and $\left(2 + P_c^{\mathrm{N}}\right) d_{\mathbf{H}} = 5.32$ Å, being unphysically small or unphysically large, respectively, can be discarded.

Because in its *trans* configuration adsorbed AB has both N atoms at the same height [31], the measured coherent fraction of N ($F_c^{\mathrm{N}} = 0.48$) is assumed to be indicative of the degree of extrinsic disorder in the molecular layer, and not related to a systematic, intrinsic distortion of the azo-bridge within each individual adsorbed molecule. The extrinsic disorder reduces the coherent fraction of each individual atom of AB to a value below 1 (ideal case) (see e.g. Ref.[13]); in particular, we have used $F_c^{\mathrm{C}_i} = F_c^{\mathrm{N}_i} = F_c^{\mathrm{N}} = 0.48$ in calculating ($P_c^{\mathrm{C}}$, $F_c^{\mathrm{C}}$)|($\omega$,$\beta$) from the atomic coordinates of step 1 by the procedure defined in section  of the present supplement.

***Ad step 3:*** Since the experimental structure parameters ($P_c^{\mathrm{C}}$, $F_c^{\mathrm{C}}$)|(exp) have error bars, a number of different ($P_c^{\mathrm{C}}$, $F_c^{\mathrm{C}}$)|($\omega$,$\beta$) fall within the experimental range, and hence a range of geometry parameters ($\omega$,$\beta$) is found to be consistent with the experimental NIXSW data. This defines the error bars of ($\omega$,$\beta$)|(exp).

Two different error bars for ($\omega$,$\beta$)|(exp), labeled *error 1* and *error 2* in the following, can be defined. The first is based on the error bars of ($P_c^{\mathrm{C}}$, $F_c^{\mathrm{C}}$) only, while the second takes into account the error bars of both ($P_c^{\mathrm{C}}$, $F_c^{\mathrm{C}}$) *and* ($P_c^{\mathrm{N}}$, $F_c^{\mathrm{N}}$) and is thus a more conservative error estimate.

Before discussing in detail how the two errors are determined, we note the following. Torsion angles $\beta$ with opposite sign but same modulus $|\beta|$ yield similar values of ($P_c^{\mathrm{C}}$, $F_c^{\mathrm{C}}$)|($\omega$, $\beta$). The AB molecule, however, is not invariant under a sign change of $\beta$ (cf. Fig. 1). Therefore, two cases must be distinguished: AB with $\beta > 0°$ and AB with $\beta < 0°$ (cf. Fig. 1a and b, respectively). Table V shows the ($\omega$, $\beta$)|(exp) in best agreement with NIXSW data separately for $\beta > 0°$ and $\beta < 0°$.

*Error 1* is determined as follows. Among the ($P_c^{\mathrm{C}}$, $F_c^{\mathrm{C}}$)|($\omega$, $\beta$) calculated using the experimental values ($d_{\mathrm{N-Ag}}$, $F_c^{\mathrm{N}}$) as described in Section , we select those within the experimental values ($P_c^{\mathrm{C}} \pm \delta P_c^{\mathrm{C}}$, $F_c^{\mathrm{C}} \pm \delta F_c^{\mathrm{C}}$) $= (0.27 \pm 0.02,\ 0.34 \pm 0.03)$. We then split the selected ($\omega$, $\beta$) into two sets, one set with $\beta > 0°$ and another one with $\beta < 0°$. Within each of the two sets we find the extremal values [($\omega_{\max}$, $\omega_{\min}$), ($\beta_{\max}$, $\beta_{\min}$)] which define *error 1* of $\omega$ and $\beta$ (Table V).

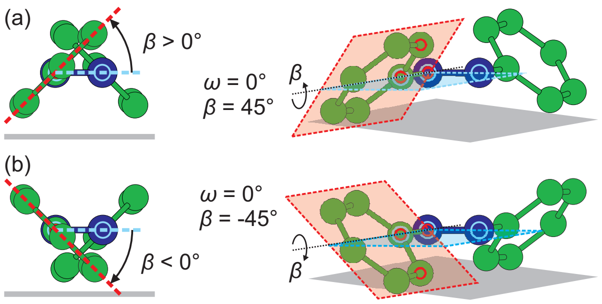


FIG. 1. (a) Side view and perspective view of AB with $\omega = 0°$ and $\beta = 45°$. (b) Side view and perspective view of AB with $\omega = 0°$ and $\beta = -45°$. $\omega$ and $\beta$ are defined in the paper. C atoms: green spheres. N atoms: blue spheres. For clarity, H atoms are not drawn.

TABLE V. $(\omega,\beta)|(\text{exp})$ with the corresponding error bars 1 and 2 (see text) for $\beta > 0°$ and $\beta < 0°$.

| | $\beta > 0°$ | | $\beta < 0°$ | |
|---|---|---|---|---|
| | $\omega$ | $\beta$ | $\omega$ | $\beta$ |
| estimate | -0.7 | 17.7 | 2.6 | -18.0 |
| *error 1* | +2.3/-2.2 | +2.4/-2.7 | +2.2/-2.3 | +2.6/-2.4 |
| *error 2* | +5.9/-4.4 | +6.8/-17.7 | +4.8/-5.5 | +18.0/-6.8 |

*Error 2* is determined as follows. The procedure described above for the determination of *error 1* is repeated for five different sets of $(P_c^{\mathrm{C}}, F_c^{\mathrm{C}})|(\omega, \beta)$ that are obtained from identical simulated AB structures, but with five different starting values $(d_{\mathrm{N-Ag}}, F_c^{\mathrm{N}})$ for the nitrogen atoms. The five starting values $(d_{\mathrm{N-Ag}}, F_c^{\mathrm{N}})$ correspond to the center and the four apexes of the error region (Fig. 2 of the paper) and are given by [(2.97 Å, 0.48), (2.92 Å, 0.60), (2.92 Å, 0.36), (3.01 Å, 0.60), (3.01 Å, 0.36)]. Hence, we obtain five corresponding intervals $[(\omega_{\max}, \omega_{\min}), (\beta_{\max}, \beta_{\min})]$ for $\beta > 0°$ and five for $\beta < 0°$. Within each set of intervals we find the extremal values which define *error 2* of $\omega$ and $\beta$ (Table V).

## NIXSW SIMULATIONS FOR DFT-CALCULATED GEOMETRIES

To simulate NIXSW structure parameters for an atomic species X $(P_c^{\mathrm{X}}, F_c^{\mathrm{X}})$ for DFT-calculated AB geometries we use the formalism reported in Section . In calculating the average coherent positions and fractions $(P_c^{\mathrm{C}}, F_c^{\mathrm{C}})$ and $(P_c^{\mathrm{N}}, F_c^{\mathrm{N}})$ of a single AB geometry,

we set in equations (5) to (12) $N_{\mathrm{C}} = 12$ (the number of carbon atoms in one molecule) and $N_{\mathrm{N}} = 2$ (the number of nitrogen atoms in one molecule).

In order to estimate the influence of AB vibrations on the coherent fractions $F_c^{\mathrm{C}}$ and $F_c^{\mathrm{N}}$, we generated a collection of 10000 AB geometries $\mathbf{R}_{210\mathrm{K},1-10000}$ mimicking the distribution due to vibrational motion at 210K. For this we took snapshots at equidistant time steps [$\Delta t = 2.25$ fs (9.36 fs) for PBE+vdW$^{\mathrm{surf}}$ (PBE+TS)] from a microcanonical molecular dynamics trajectory combining the motion of all independent vibrational modes, starting from random displacements along the latter and velocities consistent with the given temperature. In calculating the average coherent positions and fractions ($P_c^{\mathrm{C}}$, $F_c^{\mathrm{C}}$) and ($P_c^{\mathrm{N}}$, $F_c^{\mathrm{N}}$) of a collection of $N_{\mathrm{AB}}$ AB molecules we set in equations (5) to (12) $N_{\mathrm{C}} = 12N_{\mathrm{AB}}$ (the number of carbon atoms in the AB collection) and $N_{\mathrm{N}} = 2N_{\mathrm{AB}}$ (the number of nitrogen atoms in the AB collection).

Table VI reports $P_c^{\mathrm{C}}$, $F_c^{\mathrm{C}}$ and $F_c^{\mathrm{C}}/F_c^{\mathrm{N}}$ for the average AB structure at 210 K ($\mathbf{R}_{210\mathrm{K}}$) including static anharmonic corrections (cf. Section ) and for $N_{\mathrm{AB}} = 10000$ anharmonically *vibrating* AB molecules including static and dynamic corrections. We have verified that coherent positions and fractions ($P_c^{\mathrm{C}}$, $F_c^{\mathrm{C}}$) and ($P_c^{\mathrm{N}}$, $F_c^{\mathrm{N}}$) are well converged with respect to the total number of 10000 time steps that has been chosen to generate the AB collection. The percentage variation of $F_c^{\mathrm{C}}$ and $F_c^{\mathrm{N}}$ in going from the average AB structure to the AB collection is also reported in Table VI.

TABLE VI. Simulated $P_c^{\rm C}$, $P_c^{\rm N}$ and $F_c^{\rm C}/F_c^{\rm N}$ of the average AB geometry at 210 K [$\mathbf{R}_{\rm 210K}$, cf. equation (4)] and of a collection of $N_{\rm AB}$ = 10000 anharmonically *vibrating* AB molecules $\mathbf{R}_{\rm 210K,1-10000}$. Percentage variation of $F_c^{\rm C}$ ($\Delta F_c^{\rm C}$) and $F_c^{\rm N}$ ($\Delta F_c^{\rm N}$) in going from $\mathbf{R}_{\rm 210K}^{\rm AB}$ to the AB collection $\mathbf{R}_{\rm 210K,1-10000}$. Calculations were performed with PBE+TS and PBE+vdW$^{\rm surf}$ for the $(2{\rm x}5)_1$ cell (phase A) as described in Sections  and . NIXSW simulations of the DFT-calculated AB geometries were carried out as detailed in Section . Experimental $P_c^{\rm C}$, $P_c^{\rm N}$ and $F_c^{\rm C}/F_c^{\rm N}$ are also reported, along with the respective error bars.

| | | $P_c^{\rm C}$ | $P_c^{\rm N}$ | $F_c^{\rm C}/F_c^{\rm N}$ | $\Delta F_c^{\rm C}$ | $\Delta F_c^{\rm N}$ |
|---|---|---|---|---|---|---|
| TS | average AB | 0.46 | 0.35 | 0.61 | | |
| | AB collection | 0.46 | 0.35 | 0.62 | −5% | −6% |
| vdw$^{\rm surf}$ | average AB | 0.35 | 0.25 | 0.60 | | |
| | AB collection | 0.35 | 0.25 | 0.63 | −8% | −12% |
| NIXSW | | 0.27 | 0.26 | 0.71 | | |
| error | | ±0.02 | ±0.02 | | | |

* *Current address:* University of Hamburg and Center for Free-Electron Laser Science, Luruper Chausse 149, 22761 Hamburg, Germany; giuseppe.mercurio@desy.de

[1] H. J. Monkhorst and J. D. Pack, Phys. Rev. B **13**, 5188 (1976).

[2] P. Hohenberg and W. Kohn, Phys. Rev. **136**, B864 (1964).

[3] W. Kohn and L. J. Sham, Phys. Rev. **140**, A1133 (1965).

[4] S. J. Clark, M. D. Segall, C. J. Pickard, P. J. Hasnip, M. I. J. Probert,  and M. C. Refson, K. Payne, Z. Kristallogr. **220**, 567 (2005).

[5] M. C. Payne, M. P. Teter, D. C. Allan, T. A. Arias,  and J. D. Joannopoulos, Rev. Mod. Phys. **64**, 1045 (1992).

[6] D. Vanderbilt, Phys. Rev. B **41**, 7892 (1990).

[7] J. P. Perdew, K. Burke,  and M. Ernzerhof, Phys. Rev. Lett. **77**, 3865 (1996).

[8] A. Tkatchenko and M. Scheffler, Phys. Rev. Lett. **102**, 073005 (2009).

[9] E. R. McNellis, J. Meyer, and K. Reuter, Phys. Rev. B **80**, 205414 (2009).

[10] A. Tkatchenko, R. A. DiStasio, R. Car, and M. Scheffler, Phys. Rev. Lett. **108**, 236402 (2012).

[11] J. Andzelm, R. King-Smith, and G. Fitzgerald, Chem. Phys. Lett. **335**, 321 (2001).

[12] N. B. Slater, Nature **180**, 1352 (1957).

[13] G. Mercurio, O. Bauer, M. Willenbockel, N. Fairley, W. Reckien, C. H. Schmitz, B. Fiedler, S. Soubatch, T. Bredow, M. Sokolowski, and F. S. Tautz, Phys. Rev. B **87**, 045421 (2013).

[14] N. Fairley, CasaXPS, version 2.3.16, Casa Software Ltd, Bay House, 5 Grosvenor Terrace, Teignmouth, Devon TQ14 8NE, UK.

[15] G. Mercurio, *Study of Molecule-Metal Interfaces by Means of the Normal Incidence X-ray Standing Wave Technique*, Ph.D. thesis, schriften des Forschungszentrums Jülich, Reihe Schlüsseltechnologien Volume 49 (Dissertation, RWTH Aachen University, 2012) ISBN 978-3-89336-816-7, available at `http://www.fz-juelich.de/zb/juwel`.

[16] G. Mercurio, E. R. McNellis, R. J. Maurer, S. Hagen, F. Leyssner, J. Meyer, M. Wolf, P. Tegeder, S. Soubatch, K. Reuter, and F. S. Tautz, (in preparation).

[17] Torricelli is an XSW data analysis and simulation program written by G. Mercurio, copies can be obtained from s.tautz@fz-juelich.de.

[18] G. Mercurio, N. Fairley, S. Soubatch, and F. S. Tautz, (in preparation).

[19] H. E. Swanson, M. C. Morris, and E. Evans, Natl. Bur. Stand. Monogr. **25(4)**, 3 (1966).

[20] R. Kirby, T. A. Hahn, and B. D. Rothrock, American Institute of Physics Handbook, $3^{rd}$ ed., edited by D. E. Gray (McGrw-Hill, New York, 1963).

[21] V. F. Sears and S. A. Shelley, Acta Crystallogr., Sect. A **47**, 441 (1991).

[22] D. P. Woodruff, B. C. C. Cowie, and A. R. H. F. Ettema, J. Phys.: Condens. Matter **6**, 10633 (1994).

[23] G. Mercurio, E. R. McNellis, I. Martin, S. Hagen, F. Leyssner, S. Soubatch, J. Meyer, M. Wolf, P. Tegeder, F. S. Tautz, and K. Reuter, Phys. Rev. Lett. **104**, 036102 (2010).

[24] I. A. Vartanyants and J. Zegenhagen, Solid State Commun. **113**, 299 (1999).

[25] J. J. Lee, C. J. Fisher, D. P. Woodruff, M. G. Roper, R. G. Jones, and B. C. C. Cowie, Surf. Sci. **494**, 166 (2001).

[26] M. B. Trzhaskovskaya, V. I. Nefedov, and V. G. Yarzhemsky, At. Data Nucl. Data Tables **77**, 97 (2001).

[27] A. Jablonski, F. Salvat, and C. J. Powell, *NIST Electron Elastic-Scattering Cross-Section*

*Database*, Tech. Rep. (Version 3.1, National Institute of Standards and Technology, Gaithersburg, MD, 2003).

[28] A. Gerlach, F. Schreiber, S. Sellner, H. Dosch, I. A. Vartanyants, B. C. C. Cowie, T.-L. Lee, and J. Zegenhagen, Phys. Rev. B **71**, 205425 (2005).

[29] C. Stadler, S. Hansen, F. Pollinger, C. Kumpf, E. Umbach, T.-L. Lee, and J. Zegenhagen, Phys. Rev. B **74**, 035404 (2006).

[30] A. Gerlach, S. Sellner, F. Schreiber, N. Koch, and J. Zegenhagen, Phys. Rev. B **75**, 045401 (2007).

[31] E. McNellis, J. Meyer, A. D. Baghi, and K. Reuter, Phys. Rev. B **80**, 035414 (2009).
